# Supplementary material for: Membrane-mediated force transduction: Stick-slip motion of vesicles with fluid membranes
Source: arXiv:2507.07880 ancillary file (2025-07-10)
Supplement: Supplementary file 1 [file supplementary.pdf]

# Appendix

## Membrane-mediated force transduction: Stick-slip motion of vesicles with fluid membranes

Paula Magrinya<sup>a</sup>, Arin Escobar Ortiz<sup>a</sup>, Juan L. Aragones<sup>a,\*</sup> and Laura R. Arriaga<sup>a,†</sup>

<sup>a</sup> *Department of Theoretical Condensed Matter Physics,  
Condensed Matter Physics Center (IFIMAC) and Instituto Nicolás Cabrera,  
Universidad Autónoma de Madrid, 28049, Madrid, Spain*

---

\* juan.aragones@uam.es

† laura.rodriguezarriga@uam.es

## I. Supporting Figures

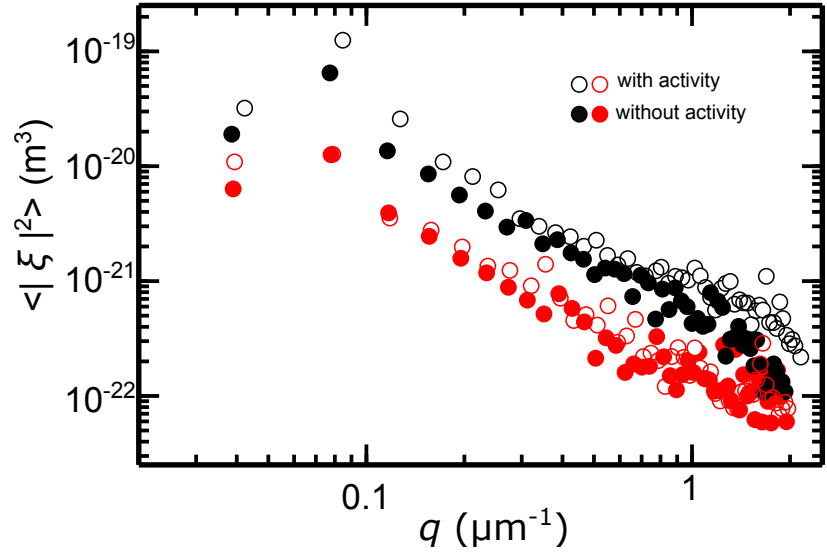

FIG. S1: Difference in the fluctuation spectrum in a vesicle encapsulating a ferromagnetic particle. Empty circles show when the particle is actuated and filled circles when it is not. Different colors represent different membrane tension.

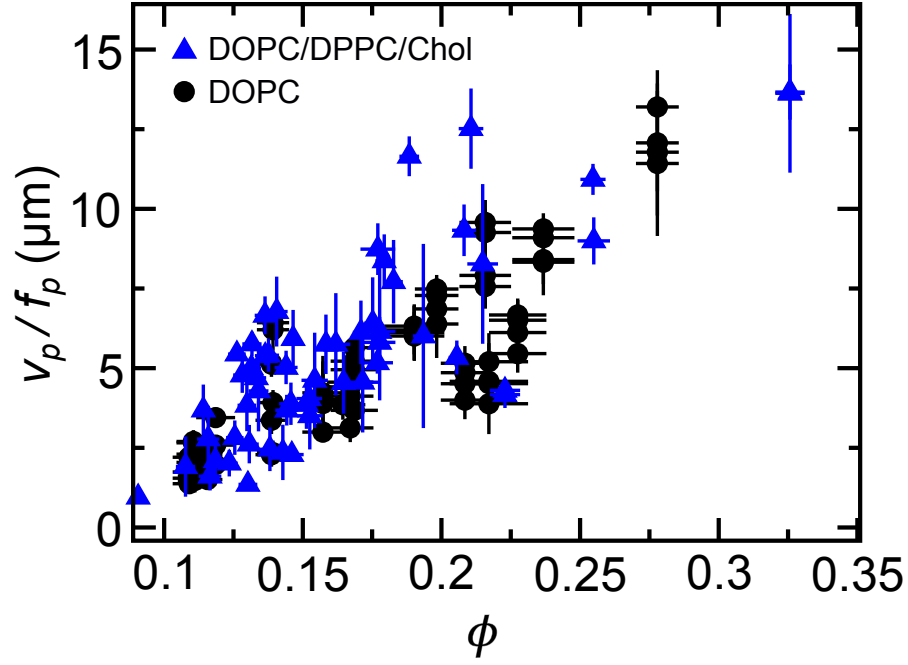

FIG. S2: Distance traveled in each particle's rotation,  $v_p/f_p$ , as a function of degree of confinement,  $\phi$ . Particle is either encapsulated in a vesicle composed of either just DOPC or a lipid mixture of DOPC/DPP/Chol.

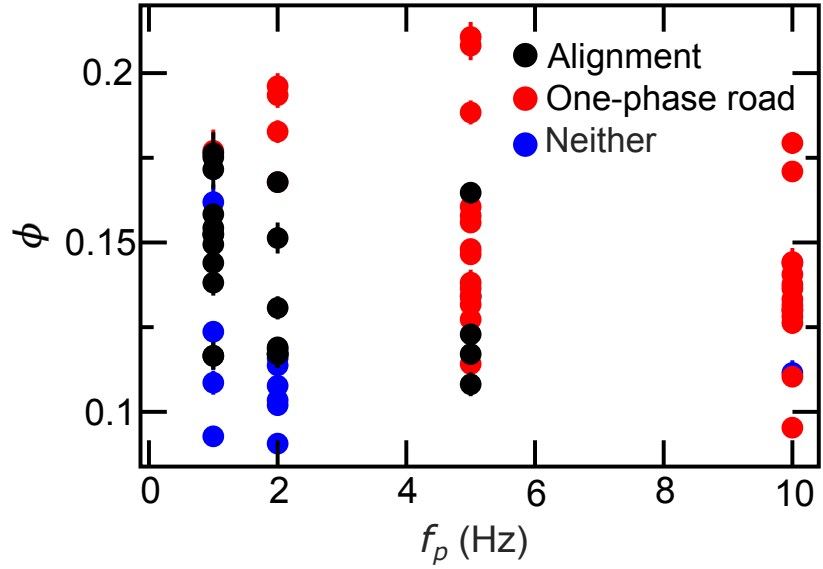

FIG. S3: Phase diagram illustrating the behavior of phase-separated vesicles, showing three distinct regions: Domain Alignment, One-Phase road, and neither of them. The diagram is plotted as a function of the degree of confinement and encapsulated particle frequency.

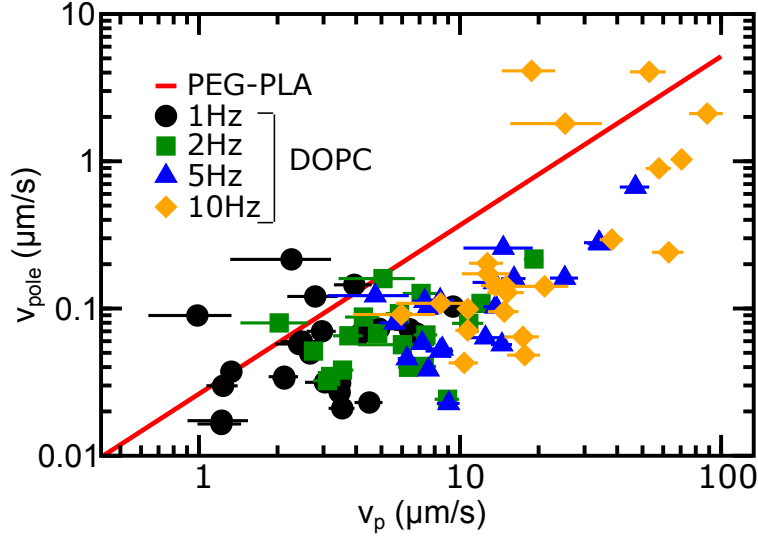

FIG. S4: Drift particle velocity towards one of the vesicles poles,  $v_{pole}$  as a function of particles velocity  $v_p$  for particles actuated at different frequencies encapsulated inside a DOPC or a PEG-PLA vesicle.

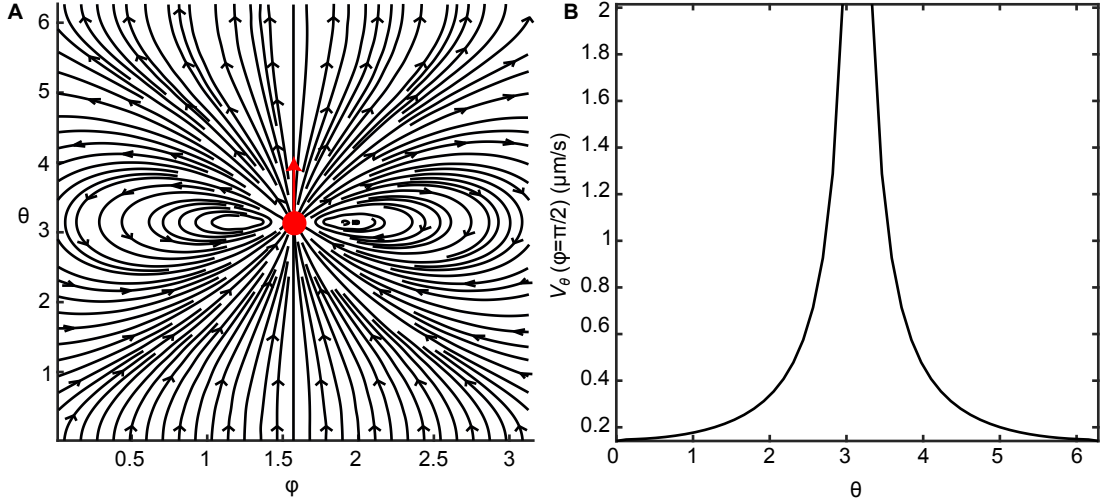

FIG. S5: A) Streamlines generated by a point force in the a vesicle membrane. B) Membrane velocity along the  $\varphi = \pi/2$  streamline. The further from the point force the smaller the velocity. Here,  $R_v = 35.5 \mu\text{m}$ ,  $F = 0.25 \text{ pN}$ ,  $\eta_m = 4 \cdot 10^{-9} \text{ Pa}\cdot\text{s}\cdot\text{m}$  and  $\eta_{3D} = 10^{-3} \text{ Pa}\cdot\text{s}$ . We have used the model described in [1].

## II. Movie Description

**Movie 1:** Behavior of a rotating particle encapsulated within a lipid vesicle (DOPC). Particle rotates with  $f_p = 2 \text{ Hz}$  and the degree of confinement is  $\phi = 0.22$ . The behavior of a free particle can also be seen.

**Movie 2:** Behavior of a rotating particle encapsulated within a phase-separated lipid vesicle (DOPC/DPPC/Chol). The particle performs diagonal movements when it encounters the domain interface,

which can be seen due to the slight budding of the vesicle. Particle rotates with  $f_p = 1$  Hz and the degree of confinement is  $\phi = 0.14$ .

**Movie 3** Alignment of domains in roller mode. Particle rotates around the  $x$ -axis and domains tilt until their boundary is perpendicular to the axis of rotation.  $f_p = 1$  Hz and  $\phi = 0.15$ .

**Movie 4** Domains rupture in roller mode. Particle forms a  $L_o$  road and performs circular loops within the road.  $f_p = 5$  Hz and  $\phi = 0.16$ .

**Movie 5** Behavior of a rotating particle encapsulated within a lipid vesicle (DOPC). The particle deviates from the equator of the vesicle and spirals towards one of the vesicle poles but fails to reach it.  $f_p = 5$  Hz and  $\phi = 0.12$ .

**Movie 6** Non uniform rotation of the vesicle's membrane. Defects (tagged in blue and black) have different rotational frequencies depending on the particle's position (tagged in magenta).  $f_p = 5$  Hz and  $\phi = 0.18$ .

---

- [1] R. Samanta and N. Oppenheimer, Vortex flows and streamline topology in curved biological membranes, *Physics of Fluids* **33**, 051906 (2021), [https://pubs.aip.org/aip/pof/article-pdf/doi/10.1063/5.0052213/19762549/051906\\_1\\_online.pdf](https://pubs.aip.org/aip/pof/article-pdf/doi/10.1063/5.0052213/19762549/051906_1_online.pdf).
